# Supplementary material for: Measurement of the top-quark production cross-section and charge asymmetry at LHCb
Source: arXiv:2512.11324 source file (2026-06-03)
Supplement: Supplementary file 1 [file supplementary.tex]

\clearpage
\section*{Supplementary material for LHCb-PAPER-2025-057}
\label{sec:Supplementary}

The total cross-sections and charge asymmetry results, compared with theoretical predictions, are shown in Figs.~\ref{fig:xsec_total} and~\ref{fig:total_asy}.
Figure~\ref{fig:mistagplot} shows the fitted $P_b$ distribution used to determine the true $b$-jet fraction.

\begin{figure}[H]
\begin{center}
\includegraphics[width=0.49\textwidth]{figs/total_xsec_mup.pdf}
\includegraphics[width=0.49\textwidth]{figs/total_xsec_mum.pdf}
\caption{Measured top-quark total cross-section compared with theoretical predictions. The bands correspond to the data. }
\label{fig:xsec_total}
\end{center}
\end{figure}

\begin{figure}[!htbp]
\begin{center}
\includegraphics[width=0.49\textwidth]{figs/total_asy.pdf}
\caption{Measured top-quark charge asymmetry compared with theoretical predictions. The bands correspond to the data.}
\label{fig:total_asy}
\end{center}
\end{figure}

\begin{figure}[!htbp]
\begin{center}
\includegraphics[width=0.5\textwidth]{figs/fiting_run2.pdf}
\caption{Distribution of  \jpb in data, fitted to determine the \bquark-jet fraction.
Also shown are stacked histograms corresponding to the contributions from $b$-, $c$-, and light-jets.
}
\label{fig:mistagplot}
\end{center}
\end{figure}

Uncertainties associated with muon identification, tracking, trigger efficiencies, jet reconstruction efficiency, event–selection efficiency, and the statistical components of the $b$-jet tagging efficiency are treated using the RMS method; the resulting correlation matrix is shown in Table~\ref{tab:corr_run2_RMS}.

All remaining systematic sources are evaluated using the envelope method.
The correlation matrix corresponding to the QCD background uncertainty obtained from the \texttt{ABCD} method is given in Table~\ref{tab:corr_run2_ABCD}. The combined background uncertainty—including contributions from the $\W+\bjet$, $\Z+\bjet$, and QCD (\texttt{ABCD}) backgrounds—is summarised in Table~\ref{tab:corr_run2_Background}, where the corresponding correlation matrix is provided.
The uncertainty from the $b$-jet tagging efficiency is treated as a fully correlated source across all $\eta_{\mu}$ bins.
The correlation matrix associated with the jet energy scale and resolution uncertainty is presented in Table~\ref{tab:corr_run2_jet_energy_scale_resolution}.
Finally, the per-bin systematic uncertainties derived from each covariance matrix are summarised in Table~\ref{tab:syst_run2}.
The uncertainties listed in this table are scaled by a factor of $10^{2}$ for clarity.

\begin{table}[!htbp]
\caption{Correlation matrix for the selection and reconstruction (RMS) uncertainties. Bins 1–4 correspond to \tquarkbar\ ($\eta_{\mu^-}$) and bins 5–8 to \tquark\ ($\eta_{\mu^+}$).}
\centering
\begin{tabular}{c|cccccccc} 
 & \multicolumn{4}{c|}{$\sigma_{\bar{t}}$ ($\eta_{\mu^-}$)} % <<< modified: added a grouped header for antitop
 & \multicolumn{4}{c}{$\sigma_{t}$ ($\eta_{\mu^+}$)} \\     % <<< modified: added a grouped header for top
\cline{2-9} % <<< modified: draws line under both multicolumn headers
Bin index & 1 & 2 & 3 & 4 & 5 & 6 & 7 & 8 \\ 
1  & $\phantom{-}$1.00 &  &  &  &  &  &  &  \\
2  & $\phantom{-}$0.75 & $\phantom{-}$1.00 &  &  &  &  &  &  \\
3  & $\phantom{-}$0.24 & $\phantom{-}$0.13 & $\phantom{-}$1.00 &  &  &  &  &  \\
4  & $-0.02$ & $\phantom{-}$0.12 & $\phantom{-}$0.14 & $\phantom{-}$1.00 &  &  &  &  \\
5  & $\phantom{-}$0.46 & $\phantom{-}$0.26 & $\phantom{-}$0.36 & $\phantom{-}$0.30 & $\phantom{-}$1.00 &  &  &  \\
6  & $\phantom{-}$0.53 & $\phantom{-}$0.45 & $\phantom{-}$0.29 & $\phantom{-}$0.15 & $\phantom{-}$0.50 & $\phantom{-}$1.00 &  &  \\
7  & $\phantom{-}$0.31 & $\phantom{-}$0.25 & $-$0.17 & $\phantom{-}$0.11 & $\phantom{-}$0.22 & $\phantom{-}$0.39 & $\phantom{-}$1.00 &  \\
8  & $-$0.07 & $\phantom{-}$0.02 & $-$0.50 & $\phantom{-}$0.14 & $\phantom{-}$0.01 & $\phantom{-}$0.05 & $\phantom{-}$0.22 & $\phantom{-}$1.00 \\
\hline
\end{tabular}
\label{tab:corr_run2_RMS}
\end{table}

\begin{table}[!htbp]
\caption{Correlation matrix for the \texttt{ABCD} method uncertainty. Bins 1–4 correspond to \tquarkbar\ ($\eta_{\mu^-}$) and bins 5–8 to \tquark\ ($\eta_{\mu^+}$). Due to the limited statistics in the last bin, the systematic uncertainties have large fluctuations, especially in the $\eta_\mu$ range 3.875–4.500.}
\centering
\begin{tabular}{c|cccccccc} 
 & \multicolumn{4}{c|}{$\sigma_{\bar{t}}$ ($\eta_{\mu^-}$)} % <<< modified: added a grouped header for antitop
 & \multicolumn{4}{c}{$\sigma_{t}$ ($\eta_{\mu^+}$)} \\     % <<< modified: added a grouped header for top
\cline{2-9} % <<< modified: draws line under both multicolumn headers
Bin index & 1 & 2 & 3 & 4 & 5 & 6 & 7 & 8 \\ 
1  & $\phantom{-}$1.00 &  &  &  &  &  &  &  \\
2  & $\phantom{-}$1.00 & $\phantom{-}$1.00 &  &  &  &  &  &  \\
3  & $-$0.79 & $-$0.79 & $\phantom{-}$1.00 &  &  &  &  &  \\
4  & $-$0.92 & $-$0.92 & $\phantom{-}$0.97 & $\phantom{-}$1.00 &  &  &  &  \\
5  & $\phantom{-}$0.99 & $\phantom{-}$0.99 & $-$0.72 & $-$0.87 & $\phantom{-}$1.00 &  &  &  \\
6  & $\phantom{-}$0.94 & $\phantom{-}$0.94 & $-$0.53 & $-$0.72 & $\phantom{-}$0.97 & $\phantom{-}$1.00 &  &  \\
7  & $-$0.01 & $-$0.01 & $\phantom{-}$0.62 & $\phantom{-}$0.41 & $\phantom{-}$0.10 & $\phantom{-}$0.34 & $\phantom{-}$1.00 &  \\
8  & $\phantom{-}$0.89 & $\phantom{-}$0.89 & $-$0.98 & $-$1.00 & $\phantom{-}$0.84 & $\phantom{-}$0.68 & $-$0.46 & $\phantom{-}$1.00 \\
\hline
\end{tabular}
\label{tab:corr_run2_ABCD}
\end{table}

\begin{table}[!htbp]
\caption{Correlation matrix for the $\W+\bjet$, $\Z+\bjet$, and QCD (\texttt{ABCD}) background uncertainty. Bins 1–4 correspond to \tquarkbar\ ($\eta_{\mu^-}$) and bins 5–8 to \tquark\ ($\eta_{\mu^+}$). Due to the limited statistics in the last bin, the systematic uncertainties have large fluctuations, especially in the $\eta_\mu$ range 3.875–4.500.}
\centering
\begin{tabular}{c|cccccccc} 
 & \multicolumn{4}{c|}{$\sigma_{\bar{t}}$ ($\eta_{\mu^-}$)} % <<< modified: added a grouped header for antitop
 & \multicolumn{4}{c}{$\sigma_{t}$ ($\eta_{\mu^+}$)} \\     % <<< modified: added a grouped header for top
\cline{2-9} % <<< modified: draws line under both multicolumn headers
Bin index & 1 & 2 & 3 & 4 & 5 & 6 & 7 & 8 \\ 
1  & $\phantom{-}$1.00 &  &  &  &  &  &  &  \\
2  & $\phantom{-}$0.11 & $\phantom{-}$1.00 &  &  &  &  &  &  \\
3  & $\phantom{-}$0.12 & $-$0.90 & $\phantom{-}$1.00 &  &  &  &  &  \\
4  & $-$0.92 & $-$0.25 & $\phantom{-}$0.16 & $\phantom{-}$1.00 &  &  &  &  \\
5  & $\phantom{-}$0.47 & $\phantom{-}$0.92 & $-$0.71 & $-$0.52 & $\phantom{-}$1.00 &  &  &  \\
6  & $\phantom{-}$0.94 & $-$0.15 & $\phantom{-}$0.43 & $-$0.74 & $\phantom{-}$0.24 & $\phantom{-}$1.00 &  &  \\
7  & $-$0.56 & $\phantom{-}$0.68 & $-$0.63 & $\phantom{-}$0.54 & $\phantom{-}$0.42 & $-$0.65 & $\phantom{-}$1.00 &  \\
8  & $\phantom{-}$0.36 & $\phantom{-}$0.88 & $-$0.88 & $-$0.60 & $\phantom{-}$0.87 & $\phantom{-}$0.03 & $\phantom{-}$0.30 & $\phantom{-}$1.00 \\
\hline
\end{tabular}
\label{tab:corr_run2_Background}
\end{table}

\begin{table}[!htbp]
\caption{Correlation matrix for the jet energy scale and resolution uncertainty. Bins 1–4 correspond to \tquarkbar\ ($\eta_{\mu^-}$) and bins 5–8 to \tquark\ ($\eta_{\mu^+}$).}
\centering
\begin{tabular}{c|cccccccc} 
 & \multicolumn{4}{c|}{$\sigma_{\bar{t}}$ ($\eta_{\mu^-}$)} % <<< modified: added a grouped header for antitop
 & \multicolumn{4}{c}{$\sigma_{t}$ ($\eta_{\mu^+}$)} \\     % <<< modified: added a grouped header for top
\cline{2-9} % <<< modified: draws line under both multicolumn headers
Bin index & 1 & 2 & 3 & 4 & 5 & 6 & 7 & 8 \\ 
1  & 1.00 &  &  &  &  &  &  &  \\
2  & 0.99 & 1.00 &  &  &  &  &  &  \\
3  & 0.98 & 1.00 & 1.00 &  &  &  &  &  \\
4  & 0.95 & 0.99 & 0.99 & 1.00 &  &  &  &  \\
5  & 1.00 & 0.99 & 0.98 & 0.95 & 1.00 &  &  &  \\
6  & 0.98 & 1.00 & 1.00 & 0.99 & 0.98 & 1.00 &  &  \\
7  & 0.95 & 0.99 & 0.99 & 1.00 & 0.95 & 0.99 & 1.00 &  \\
8  & 0.91 & 0.96 & 0.97 & 0.99 & 0.90 & 0.97 & 0.99 & 1.00 \\
\hline
\end{tabular}
\label{tab:corr_run2_jet_energy_scale_resolution}
\end{table}

\begin{table}[!htbp]
\centering
\caption{Per-bin systematic uncertainties for the \tquarkbar and \tquark
differential cross-section measurements. The uncertainties are quoted in units of \pb. The numerical values shown in the table have been scaled by a factor of $10^{2}$. Bins 1–4 correspond to \tquarkbar\ ($\eta_{\mu^-}$) and bins 5–8 to \tquark\ ($\eta_{\mu^+}$).}
\begin{tabular}{c|cccccccc}
 & \multicolumn{4}{c|}{$\sigma_{\bar{t}}$ ($\eta_{\mu^-}$)} % <<< modified: added a grouped header for antitop
 & \multicolumn{4}{c}{$\sigma_{t}$ ($\eta_{\mu^+}$)} \\     % <<< modified: added a grouped header for top
\cline{2-9} % <<< modified: draws line under both multicolumn headers
Bin index & 1 & 2 & 3 & 4 & 5 & 6 & 7 & 8 \\ \hline
RMS & 0.37 & 0.25 & 0.16 & 0.06 & 0.38 & 0.28 & 0.16 & 0.09 \\
$b$-jet tagging & 3.90 & 2.66 & 1.14 & 0.33 & 4.70 & 3.20 & 1.48 & 0.46 \\
Jet energy scale and resolution & 3.27 & 2.14 & 0.80 & 0.21 & 3.66 & 2.61 & 1.17 & 0.35 \\
\texttt{ABCD} & 1.59 & 0.90 & 0.42 & 0.47 & 1.81 & 0.62 & 0.14 & 0.42 \\
$\W+\bjet$ and $\Z+\bjet$ background & 2.01 & 1.31 & 0.72 & 0.53 & 1.99 & 1.00 & 0.44 & 0.47 \\
Total systematic & 5.49 & 3.67 & 1.57 & 0.66 & 6.29 & 4.26 & 1.95 & 0.75 \\
\hline
\end{tabular}
\label{tab:syst_run2}
\end{table}
